# Supplementary material for: OmniDet: Surround View Cameras based Multi-task Visual Perception Network for Autonomous Driving
Source: arXiv:2102.07448 source file (2023-06-06)
Supplement: Supplementary file 1 [file supplementary.tex]

% -------------------------------------------------
\begin{table*}[htpb]
\centering
\captionsetup{belowskip=-12pt, font= small, singlelinecheck=false}
\scalebox{1.25}{
\begin{tabular}{ll}
\toprule
$\textbf{Abs Rel}: \frac{1}{|N|}\sum_{i\in N}\frac{\mid d_{i}-d_{i}^{*}\mid}{d_{i}^{*}}$
&$\textbf{RMSE}:\sqrt{\frac{1}{|N|}\sum_{i\in N}\parallel d_{i}-d_{i}^{*} \parallel^{2}}$\\
$\textbf{Sq Rel}:\frac{1}{|N|}\sum_{i\in N}\frac{\parallel d_{i}-d_{i}^{*}\parallel^{2}}{d_{i}^{*}}$
&$\textbf{RMSE log}: \sqrt{\frac{1}{|N|}\sum_{i\in N}\parallel \log (d_{i})- \log (d_{i}^{*}) \parallel^{2}}$ \\
\multicolumn{2}{l}{\textbf{Accuracies} $\mathbf{\delta}_\mathbf{t}:
\frac{1}{|N|}|\{d \in N| \: \max(\frac{d_{i}}{d_{i}^{*}}, \frac{d_{i}^{*}}{d_{i}}) \: < 1.25^t\}|\times 100\%$} \\
\bottomrule
\end{tabular}
}
\caption{Performance indicators for depth evaluation. where $d_{i}$ and  $d_{i}^{*}$ denotes the predicted and ground truth depth value of pixel $i$ respectively. $N$ denotes the set of a total number of pixels with real-depth/distance values in an image, $|.|$ returns the number of the input set elements.}
\end{table*}
% -------------------------------------------------
\begin{table*}[!ht]
\captionsetup{belowskip=-12pt, font= small, singlelinecheck=false}

\centering
{
\small
\setlength{\tabcolsep}{0.3em}
\begin{tabular}{c|llccccccc}
\toprule
& \multirow{2}{*}{\textbf{Method}}
& Train
& \cellcolor[HTML]{5880ab}Abs Rel & \cellcolor[HTML]{5880ab}Sq Rel & \cellcolor[HTML]{5880ab}RMSE & \cellcolor[HTML]{5880ab}RMSE$_{log}$ & \cellcolor[HTML]{e8715b}$\delta<1.25$ & \cellcolor[HTML]{e8715b}$\delta<1.25^2$ & \cellcolor[HTML]{e8715b}$\delta<1.25^3$ \\
\cmidrule(lr){4-7} \cmidrule(lr){8-10}
& & & \multicolumn{4}{c}{\cellcolor[HTML]{5880ab}lower is better} & \multicolumn{3}{c}{\cellcolor[HTML]{e8715b}higher is better} \\
\toprule
\parbox[t]{2mm}{\multirow{33}{*}{\rotatebox[origin=c]{90}{Original~\cite{Eigen_14}}}}
& SfMLearner~\cite{zhou2017unsupervised}      & M & 0.208 & 1.768 & 6.958 & 0.283 & 0.678 & 0.885 & 0.957 \\
& DNC~\cite{yang2017unsupervised}             & M & 0.182 & 1.481 & 6.501 & 0.267 & 0.725 & 0.906 & 0.963 \\
& Vid2Depth~\cite{mahjourian2018unsupervised} & M & 0.163 & 1.240 & 6.220 & 0.250 & 0.762 & 0.916 & 0.968 \\
& LEGO~\cite{yang2018lego}                    & M & 0.162 & 1.352 & 6.276 & 0.252 & 0.783 & 0.921 & 0.969 \\
& Kumar~\cite{Kumar2018a}                & M & 0.211 & 1.979 & 6.154 & 0.263 & 0.731 & 0.897 & 0.959 \\
& Wang \etal~\cite{wang2019unsupervised}      & M & 0.158 & 1.277 & 5.858 & 0.233 & 0.785 & 0.929 & 0.973 \\
& GeoNet~\cite{Yin2018}                       & M & 0.155 & 1.296 & 5.857 & 0.233 & 0.793 & 0.931 & 0.973 \\
& Cycle-SfM~\cite{sun2019cycle}               & M & 0.162 & 1.349 & 5.847 & 0.239 & 0.784 & 0.925 & 0.969 \\
& Li \etal~\cite{li2019sequential}            & M & 0.150 & 1.127 & 5.564 & 0.229 & 0.823 & 0.936 & 0.974 \\
& DDVO~\cite{Wang2018e}                & M & 0.151 & 1.257 & 5.583 & 0.228 & 0.810 & 0.936 & 0.974 \\
& DF-Net~\cite{zou2018df}                     & M & 0.150 & 1.124 & 5.507 & 0.223 & 0.806 & 0.933 & 0.973 \\
& GANVO~\cite{almalioglu2019ganvo}            & M & 0.150 & 1.141 & 5.448 & 0.216 & 0.808 & 0.939 & 0.975 \\
& Bian~\cite{bian2019unsupervised}            & M & 0.137 & 1.089 & 5.439 & 0.217 & 0.830 & 0.942 & 0.975 \\
& EPC++~\cite{Yang2018c}                      & M & 0.141 & 1.029 & 5.350 & 0.216 & 0.816 & 0.941 & 0.976 \\
& CC~\cite{Ranjan2019}             & M & 0.140 & 1.070 & 5.326 & 0.217 & 0.826 & 0.941 & 0.975 \\
& Struct2Depth~\cite{Casser2019}              & M & 0.141 & 1.036 & 5.291 & 0.215 & 0.816 & 0.945 & 0.979 \\
& LearnK~\cite{Gordon2019}                    & M & 0.128 & 0.959 & 5.230 & 0.212 & 0.845 & 0.947 & 0.976 \\
& SIGNet~\cite{Meng2019a}                & M & 0.133 & 0.905 & 5.181 & 0.208 & 0.825 & 0.947 & 0.981 \\
& DualNet~\cite{Zhou2019}                     & M & 0.121 & 0.837 & 4.945 & 0.197 & 0.853 & 0.955 & 0.982 \\
& OmegaNet~\cite{tosi2020distilled}           & M & 0.126 & 0.835 & 4.937 & 0.199 & 0.844 & 0.953 & 0.982 \\
& SuperDepth~\cite{pillai2019superdepth}      & M & 0.116 & 1.055 & -     & 0.209 & 0.853 & 0.948 & 0.977 \\
& Monodepth2~\cite{Godard2019}                & M & 0.115 & 0.903 & 4.863 & 0.193 & 0.877 & 0.959 & 0.981 \\
& PackNet-SfM~\cite{Guizilini2020a}           & M & 0.111 & 0.829 & 4.788 & 0.199 & 0.864 & 0.954 & 0.980 \\
& FisheyeDistanceNet~\cite{kumar2019fisheyedistancenet} & M & 0.117 & 0.867 & 4.739 & 0.190 & 0.869 & 0.960 & 0.982 \\
& SGDepth~\cite{Klingner2020}                 & M & 0.113 & 0.880 & 4.695 & 0.192 & 0.884 & 0.961 & 0.981 \\
& Patil \etal~\cite{patil2020don}             & M & 0.111 & 0.821 & 4.650 & 0.187 & 0.883 & 0.961 & 0.982 \\
& UnRectDepthNet~\cite{kumar2020unrectdepthnet} & M & 0.107 & 0.721 & 4.564 & 0.178 & 0.894 & 0.971 & 0.986 \\
& SynDistNet~\cite{kumar2020syndistnet}       & M & 0.109 & 0.718 & 4.516 & 0.180 & 0.896 & 0.973 & 0.986 \\
& Shu \etal~\cite{shu2020featdepth}           & M & 0.104 & 0.729 & 4.481 & 0.179 & 0.893 & 0.965 & 0.984 \\
& OmniDet                                     & M & \textbf{0.092} & \textbf{0.657} & \textbf{3.984} & \textbf{0.168} & \textbf{0.914} & \textbf{0.975} & \textbf{0.986} \\
\cmidrule{2-10}
& Struct2Depth~\cite{Casser2019}             & M${^*}$ & 0.109 & 0.825 & 4.750 & 0.187 &0.874 & 0.958 & 0.983 \\
& GLNet~\cite{Chen2019b}                     & M$^{*}$ & 0.099 & 0.796 & 4.743 & 0.186 &0.884 & 0.955 & 0.979 \\
& Shu \etal~\cite{shu2020featdepth}          & M$^{*}$ & 0.088 & 0.712 & 4.137 & \textbf{0.169} & 0.915 & 0.965 & 0.982 \\
& OmniDet                                    & M$^{*}$ & \textbf{0.077} & \textbf{0.641} & \textbf{3.859} & \textbf{0.152} & \textbf{0.931} & \textbf{0.979} & \textbf{0.989} \\
\midrule
\parbox[t]{2mm}{\multirow{11}{*}{\rotatebox[origin=c]{90}{Improved~\cite{uhrig2017sparsity}}}}
& SfMLearner~\cite{zhou2017unsupervised}    & M & 0.176 & 1.532 & 6.129 & 0.244 & 0.758 & 0.921 & 0.971 \\
& Vid2Depth~\cite{mahjourian2018unsupervised} & M & 0.134 & 0.983 & 5.501 & 0.203 & 0.827 & 0.944 & 0.981 \\
& GeoNet~\cite{Yin2018}                     & M & 0.132 & 0.994 & 5.240 & 0.193 & 0.883 & 0.953 & 0.985 \\
& DDVO~\cite{Wang2018e}              & M & 0.126 & 0.866 & 4.932 & 0.185 & 0.851 & 0.958 & 0.986 \\
& EPC++~\cite{Yang2018c}                    & M & 0.120 & 0.789 & 4.755 & 0.177 & 0.856 & 0.961 & 0.987 \\
& Monodepth2~\cite{Godard2019}              & M & 0.090 & 0.545 & 3.942 & 0.137 & 0.914 & 0.983 & 0.995 \\
& PackNet-SfM~\cite{Guizilini2020a}         & M & 0.078 & 0.420 & 3.485 & 0.121 & 0.931 & 0.986 & 0.996 \\
& UnRectDepthNet~\cite{kumar2020unrectdepthnet} & M & 0.081 & 0.414 & 3.412 & 0.117 & 0.926 & 0.987 & 0.996 \\
& SynDistNet~\cite{kumar2020syndistnet}     & M & 0.076 & 0.412 & 3.406 & 0.115 & 0.931 & 0.988 & 0.996 \\
& OmniDet                                   & M  & \textbf{0.067} & \textbf{0.306} & \textbf{3.098} & \textbf{0.101} & \textbf{0.944} & \textbf{0.991} & \textbf{0.997} \\
& OmniDet                                   & M$^{*}$ & \textbf{0.048} & \textbf{0.287} & \textbf{2.913} & \textbf{0.081} & \textbf{0.948} & \textbf{0.991} & \textbf{0.998} \\
\bottomrule
\end{tabular}
}
\caption{\textbf{Evaluation of the KITTI Eigen split} compared to most of the previous self-supervised monocular depth estimation methods. Following best practices, we cap depths at 80\,m. We also evaluate using the \textit{Original} depth maps generated from raw point clouds as proposed by \cite{Eigen_14} as well as \textit{Improved} annotated depth maps as introduced by \cite{uhrig2017sparsity}. M indicates that sequences are trained on using the monocular approach. M${^*}$ indicates the online refinement technique~\cite{Casser2019}, where the model is trained during the inference. Note that while most approaches use median scaling concerning the ground truth at test-time for a scale-consistent prediction, we do not need to use this scaling method.}
\label{tab:kitti-monocular-results}
\end{table*}
% -------------------------------------------------
