# Supplementary material for: OmniDet: Surround View Cameras based Multi-task Visual Perception Network for Autonomous Driving
Source: arXiv:2102.07448 source file (2023-06-06)
Supplement: Supplementary file 3 [file metrics_formulas.tex]

\begin{table*}[htpb]
\centering
\captionsetup{belowskip=-12pt, font= small, singlelinecheck=false}
\scalebox{1.25}{
\begin{tabular}{ll}
\toprule
$\textbf{Abs Rel}: \frac{1}{|N|}\sum_{i\in N}\frac{\mid d_{i}-d_{i}^{*}\mid}{d_{i}^{*}}$
&$\textbf{RMSE}:\sqrt{\frac{1}{|N|}\sum_{i\in N}\parallel d_{i}-d_{i}^{*} \parallel^{2}}$\\
$\textbf{Sq Rel}:\frac{1}{|N|}\sum_{i\in N}\frac{\parallel d_{i}-d_{i}^{*}\parallel^{2}}{d_{i}^{*}}$
&$\textbf{RMSE log}: \sqrt{\frac{1}{|N|}\sum_{i\in N}\parallel \log (d_{i})- \log (d_{i}^{*}) \parallel^{2}}$ \\
\multicolumn{2}{l}{\textbf{Accuracies} $\mathbf{\delta}_\mathbf{t}:
\frac{1}{|N|}|\{d \in N| \: \max(\frac{d_{i}}{d_{i}^{*}}, \frac{d_{i}^{*}}{d_{i}}) \: < 1.25^t\}|\times 100\%$} \\
\bottomrule
\end{tabular}
}
\caption{Performance indicators for depth evaluation. where $d_{i}$ and  $d_{i}^{*}$ denotes the predicted and ground truth depth value of pixel $i$ respectively. $N$ denotes the set of a total number of pixels with real-depth/distance values in an image, $|.|$ returns the number of the input set elements.}
\end{table*}
